# Supplementary material for: Security Implications Of Compiler Optimizations On Cryptography -- A Review
Source: arXiv:1907.02530 source file (2019-07-04)
Supplement: Supplementary file 1 [file appendix.tex]

\pagebreak
\appendix
\section{Appendix}

\subsection{Dead Store Elimination}
\label{appdse}

\begin{lstlisting}[language=c,caption=C Code]
int dummy(int x){
  int y = x+1;
  return y;
}

int secret_function(){
  int key = 0xDEADBEEF;
  int y = dummy(key);
  key = 0x00; // <---- Missing in assembly code
  return y;
}
\end{lstlisting}

\begin{lstlisting}[caption=Assembly Code]
; clang 3.9 -O1  -m32 -march=i386
dummy(int):
mov     eax, dword ptr [esp + 4]
inc     eax
ret

secret_function():
sub     esp, 12
mov     dword ptr [esp], -559038737
call    dummy(int)
add     esp, 12 ; <---- Missing mov 0 (Optimized)
ret
\end{lstlisting}

\newpage

\subsection{Constant-Time Selection Problem}
\label{appconst}

\begin{lstlisting}[language=c,caption=C Code]
int conditional_select(bool b, int x, int y){
  if(b){
    return x;
  } else {
    return y;
  }
}
\end{lstlisting}

\begin{lstlisting}[caption=Assembly Code]
; clang 3.9 -O3  -m32 -march=i386
conditional_select(bool, int, int):
mov     al, byte ptr [esp + 4]
test    al, al
jne     .LBB0_1  ; <--- JUMP
lea     eax, [esp + 12]
mov     eax, dword ptr [eax]
ret
.LBB0_1:
lea     eax, [esp + 8]
mov     eax, dword ptr [eax]
ret
\end{lstlisting}
